# Supplementary material for: Compilation Techniques for Graph Algorithms on GPUs
Source: arXiv:2012.07990 source file (2021-01-08)
Supplement: Supplementary file 1 [file appendix.tex]

\section{Appendix}
\label{sec:appendix}

\begin{figure}
    \centering
    \begin{lstlisting} [language=graphit,escapechar=|,morekeywords={[4],Function,VertexSet,AtomicCompareAndSwap, EnqueueVertex,WhileLoopStmt,EdgeSetIterator,VertexSetSize,If,AssignStmt,HybridOperator}]
...
Function updateEdge (int32_t src, int32_t dst, 
    VertexSet output_frontier, {
    bool enqueue = AtomicCompareAndSwap(parent[dst], -1, src), 
    If (enqueue, {
        EnqueueVertex<format=SPARSE>(output_frontier, dst)
    }, {})
})
Function updateEdge2 (int32_t src, int32_t dst, 
    VertexSet output_frontier, {
    AssignStmt(parent[dst], src),
    EnqueueVertex<format=bitmap>(output_frontier, dst)
})
Function main (int32_t argc, char* argv[], {
    ...
    WhileLoopStmt<needs_fusion=false>(VertexSetSize(frontier), {
        HybridOperator<runtime_threshold=true>(
            INPUT_VERTEX_SET_SIZE, "argv[3]", {
            EdgeSetIterator<requires_output=true, 
                can_reuse_frontier=true, 
                direction=PUSH, 
                is_edge_parallel=true>(
                edges, frontier, output, updateEdge, toFilter)
        }, {
            EdgeSetIterator<requires_output=true, 
                can_reuse_frontier=true, 
                direction=PULL, 
                is_edge_parallel=false>(
                edges, frontier, output, updateEdge2, toFilter)
        }), 
        AssignStmt(frontier, output)
    }),
    ...
})
    \end{lstlisting}
    \caption{The \graphisa generated by the compiler for the \bfs algorithm and the schedule in Figure~\ref{lst:bfs_schedule1}. Parameters to instruction are specified in \lstinline{()} and metadata is specified in \lstinline{<>}. Some of the metadata is omitted for brevity.}
    \label{fig:bfs_isa1}
\end{figure}
